# Supplementary material for: Black-Box Policy Search with Probabilistic Programs
Source: arXiv:1507.04635 source file (2016-08-04)
Supplement: Supplementary file 1 [file mdpp-supplement.tex]

\documentclass[twoside]{article}
\usepackage[accepted]{aistats2016}
\usepackage{natbib}
\usepackage{amsmath}
\usepackage{amssymb}
\usepackage{hyperref}
\usepackage{url}
\usepackage[]{graphicx}
\usepackage{verbatim}
\usepackage{listings}
\usepackage{rotating}
\usepackage[scale=0.9]{sourcecodepro}

\usepackage{microtype}

\usepackage{caption}
\setlength{\floatsep}{5pt plus 2pt minus 2pt}
\setlength{\intextsep}{5pt plus 2pt minus 2pt}

\usepackage{algorithm}
\usepackage{algpseudocode}

\input{macros.tex}
\input{anglican.tex}

\lstset{language=Anglican,basicstyle=\footnotesize\ttfamily,showstringspaces=false}

\begin{document}
\onecolumn

%{\twocolumn[
\aistatstitle{Supplemental~Material~for Black-Box~Policy~Search~with~Probabilistic~Programs}

\aistatsauthor{Jan-Willem van de Meent \And Brooks Paige \And David Tolpin \And Frank Wood }

\aistatsaddress{ Department of Engineering Science, University of Oxford}
%]}
%
%Test
%
%\onecolumn
%
%Test two

\appendix
\input{appendix.tex}

\end{document}
